# Supplementary material for: RoboTwin: Dual-Arm Robot Benchmark with Generative Digital Twins (early version)
Source: arXiv:2409.02920 source file (2025-04-16)
Supplement: Supplementary file 1 [file appendix.tex]

\appendix
\section{Appendix}
\subsection{Licensing}
RoboTwin is released under the open-source MIT license.

\subsection{Benchmark Task Descriptions}
\label{sup:Benchmark Task Descriptions}
In this subsection, we present a comprehensive overview of six carefully designed simulation tasks aimed at evaluating the capabilities of robotic systems in various manipulation scenarios. These tasks are crafted to challenge different aspects of dexterous control, coordination between multiple limbs, and the ability to perform complex sequences of actions. Each task is intended to simulate real-world challenges that a robotic system might encounter, thus providing a robust benchmark for assessing the effectiveness of various robotic algorithms. Detailed descriptions of these tasks are provided in Table \ref{tab:benchmark_description}, which outlines the specific objectives and required actions for each scenario.

\begin{longtable}{>{\itshape\centering}m{3.5cm} p{8cm}}
\caption{Detailed descriptions of 6 simulation tasks we propose.}
\label{tab:benchmark_description} \\
\toprule
\textbf{Task}   & \textbf{Description}        \\ \midrule 
\endfirsthead

\multicolumn{2}{c}%
{{\bfseries \tablename\ \thetable\ -- continued from previous page}} \\
\toprule
\textbf{Task}   & \textbf{Description}        \\ \midrule 
\endhead

\multicolumn{2}{r}{{Continued on next page}} \\ \bottomrule
\endfoot

\bottomrule
\endlastfoot

Block Hammer Beat & A hammer and a red block are on the table. The right arm uses the hammer to strike the block.                                               \\ \midrule
Empty Cup Place & A cup (without liquid) is on the table. The right arm picks up the cup from above downwards and places it on a cup mat.                         \\ \midrule

Dual-Bottles Pick & The left arm grasps a cola can, while the right arm simultaneously picks up a sprite can.                                     \\ \midrule
Block Sweep & There is a red block on the table. The left arm of the robotic arm holds the dustpan and the right arm holds the brush. The two arms work together to sweep the block in. \\ \midrule
Apple Cabinet Storage & On the table, there's a cabinet and an apple. The left arm opens the cabinet, and the right arm picks up the apple, placing it inside.         \\ \midrule
Block Handover & The left arm picks up the red cuboid on the left side of the desk and hands it over to the right arm, which will then place the cuboid in the blue target area on the right side.                                     \\
\end{longtable}

\subsection{Dataset Task Descriptions}
\label{sup:Dataset Task Descriptions}

Our dataset comprises 17 distinct, real-world robotic tasks designed to evaluate the dexterity, coordination, and contextual understanding of robotic systems in a controlled environment. Each task is uniquely structured to challenge various aspects of robotic manipulation, from simple object transfers to complex, dual-arm coordination tasks. Table \ref{tab:dataset_description} provides detailed descriptions of each task, outlining the specific actions, objects, and expected interactions. These descriptions are pivotal for replicating the tasks in different research settings, ensuring consistency in performance benchmarks across various robotic platforms. The diverse nature of these tasks enables comprehensive testing of the robots' abilities to handle real-world scenarios, thereby advancing our understanding and development of more adaptive and capable robotic assistants.

\begin{longtable}{>{\itshape\centering}m{3.5cm} p{8cm}}
\caption{Detailed descriptions of 17 real-world tasks we propose.}
\label{tab:dataset_description} \\
\toprule
\textbf{Task}   & \textbf{Description}                                                                                                        \\ \midrule 
\endfirsthead

\multicolumn{2}{c}%
{{\bfseries \tablename\ \thetable\ -- continued from previous page}} \\
\toprule
\textbf{Task}   & \textbf{Description}                                                                                                        \\ \midrule 
\endhead

\multicolumn{2}{r}{{Continued on next page}} \\ \bottomrule
\endfoot

\bottomrule
\endlastfoot

Paddle Sweep & On the table, there is a dustpan, a brush, and a ping pong ball. Using the left arm to grasp the dustpan and the right arm to grasp the brush, the two arms work together to sweep the ping pong ball into the dustpan.  \\ \midrule
Mark Hammer Beat & A hammer and a red mark are on the table. The right arm picks up the hammer and strikes the mark.                                               \\ \midrule
Flour Scoop & On the table, there is a bowl full of flour and an empty plate. The right arm initially holds a spoon, scoops a spoonful of flour from the bowl, and then pours it into the empty plate. \\ \midrule
Brush Adjust & A brush is on the table. The left arm first picks up the brush, and the right arm adjusts the brush's position.                                 \\ \midrule
Plate Scrub & A dishrag and a plate are on the table. The left arm picks up the plate, and the right arm picks up the dishrag. The two arms work together to scrub the plate with the dishrag for three circles. \\ \midrule
Pot Wire Scrub & A stainless steel pot and a steel wool pad are on the table. The left arm adjusts the position of the pot, and the right arm picks up the steel wool pad. \\ \midrule
Cake Fork & A small plate with a piece of cake is on the table. Initially, the right arm holds a fork, and it uses the fork to pierce the cake and lift it. \\ \midrule
Stain Clean & There is a juice stain on the table with a rag. The right arm picks up the rag and wipes away the juice.                                        \\ \midrule
Scissors Take & A human is holding the head of the scissors. The right arm grabs the handle of the scissors and takes them over.                                \\ \midrule
Pot Handover & A human is holding the pot with both hands. The robot arms work together to grab the pot's handles and transfer the pot to the table.           \\ \midrule
Empty Cup Place & A cup (without liquid) is on the table. The right arm picks up the cup from above downwards and places it on a cup mat.                         \\ \midrule
Empty Cup Handover & A water cup (without liquid) is on the table. The right arm grasps the cup from above downwards and hands it over to a human.                   \\ \midrule
Empty Cup Transfer & A human is holding a cup (without liquid). The right arm picks up the cup from above downwards and transfers it to a cup mat.                   \\ \midrule
Water Cup Place & A cup with water is on the table. The right arm picks up the cup from the side and places it on a cup mat.                                      \\ \midrule
Juice Cup Transfer & A human is holding a cup with juice. The right arm picks up the cup from the side and transfers it to a cup mat.                                \\ \midrule
Juice Cup Place & A cup with juice is on the table. The right arm picks up the cup from the side and places it on a cup mat.                            \\ \midrule
Dual-Bottles Pick & The left arm grasps a cola can, while the right arm simultaneously picks up a sprite can.   \\
\end{longtable}
